# Supplementary material for: "Because Some Sighted People, They Don't Know What the Heck You're Talking About:" A Study of Blind TikTokers' Infrastructuring Work to Build Independence
Source: arXiv:2310.07154 source file (2023-12-11)
Supplement: Supplementary file 1 [file 9_Appendix.tex]

\appendix
\label{appendix}

\section{Interview Protocol}

\subsection{Introduction}
Hello, we are human-computer interaction researchers from [Institution Name]. We are trying to understand how people with visual impairments use TikTok. We will conduct an interview with you. In the interview, you are free to skip or refuse to answer any question, you can also quit the interview at any time you want. The interview will be audio-recorded and all the information will only be used for research purposes. We will replace all identifiable information like name, address, etc when we report our study. Can we start now?

\subsection{Interview Questions}

\begin{enumerate}
 \item Why do you use TikTok?
  \begin{itemize}
  \item Using TikTok for Communication?
  \item Using TikTok for Fun?
  \item Or other purposes?
  \end{itemize}

\item How is the overall experience of using TikTok?

\item Are there any differences between TikTok and other social media platforms (YouTube, Twitter, Instagram, Facebook)?
  \begin{itemize}
  \item short video vs long video?
  \item video vs text/image
  \item mobile phone vs computer?
  \end{itemize}

\item What content do you upload to TikTok? 
  \begin{itemize}
  \item any common topics of your videos?
  \item any difference from content posted on other social media?
  \end{itemize}

\item How do you create TikTok videos? 
  \begin{itemize}
  \item how to take a video/ make clips/ add BGM/ add caption/ choose a filter?
  \item any considerations for your audience who are also PVI?
  \item what do you do to increase the number of viewers?
  \item how do you interact with your audience?
  \end{itemize}

\item How do you host TikTok live-streamings? 
  \begin{itemize}
  \item how to invite people to your live-streaming?
  \item how to interact with the viewers?

\item What 
  \end{itemize}

\end{enumerate}

How do you do Live Stream? (do you need to rely on some tech or person)
What functions do you use?
What other apps or devices do you use to live stream?
Do you use smart speakers while doing a live stream
How to deal with too many live comments
What do you do to increase the number of viewers?

With Content Moderator
“Common questions answered on the homepage”
Do anything to avoid censorship or content moderation?
Have you ever experienced content moderation? When experiencing content moderation,
Have you ever tried to avoid moderation? Can you give me an example?
What are the methods you tried?
What are the features/functions you used to support your circumvention?
Have you ever tried to contact TikTok about this problem?
 If yes, can you describe the report process?
    How do you feel about the process? Do you get feedback from the platform?
What do you think TikTok should do to improve the moderation mechanism?

Appearance (do you need to rely on some tech or person)
Do you do make-up or dressing before you make TikTok content?
Why
How
Any aspect you pay attention to when you do make-up or dress?
Do TikTok alone or with the help of close social networks
Who do you ask for help?
How did they help?
Any occasions that you don’t want help or they are not so helpful?
Social Interactions
What content do you consume on TikTok?
What comments you will say? How to leave comments?
What content you would “Like” them?
What comments did you get?
How did you reply to them?
Have you ever used the “Reply comments with previous videos” function?
Sharing content with others? (Do you feel supported by them?)
With whom? 
How to share?
Collaboration on TikTok Video or Live Stream Shows?
With whom?
What kind of collaboration was it?
How was the experience?
Using any special devices or technology
Monetizing TikToks
How to increase your revenue through TikToks
Where did you learn the strategies or techniques of monetizing TikTok?
What’s the favorite video/live stream you’ve created on TikTok?
A favorite live show you’ve given?
Comments you received?
What’s the favorite video/live stream you’ve watched
A favorite live show you’ve consumed?
Comments you gave?
Get any friends from TikTok?
How did you know each other?
Is the person also visually impaired?
Others
Challenges of using TikTok?
How did you overcome them?
Can I use some of the videos’ quotes in our study?
